# Supplementary material for: MatIR: A Hybrid Mamba-Transformer Image Restoration Model
Source: arXiv:2501.18401 source file (2025-01-31)
Supplement: Supplementary file 1 [file X_suppl.tex]

% \clearpage
\setcounter{section}{0}
\setcounter{table}{0}
\setcounter{figure}{0}

\maketitlesupplementary

\begin{figure*}
    \centering
    
    \captionsetup{font={small}} 
    
    \includegraphics[width=.99\linewidth]{arXiv-2311.11600v1/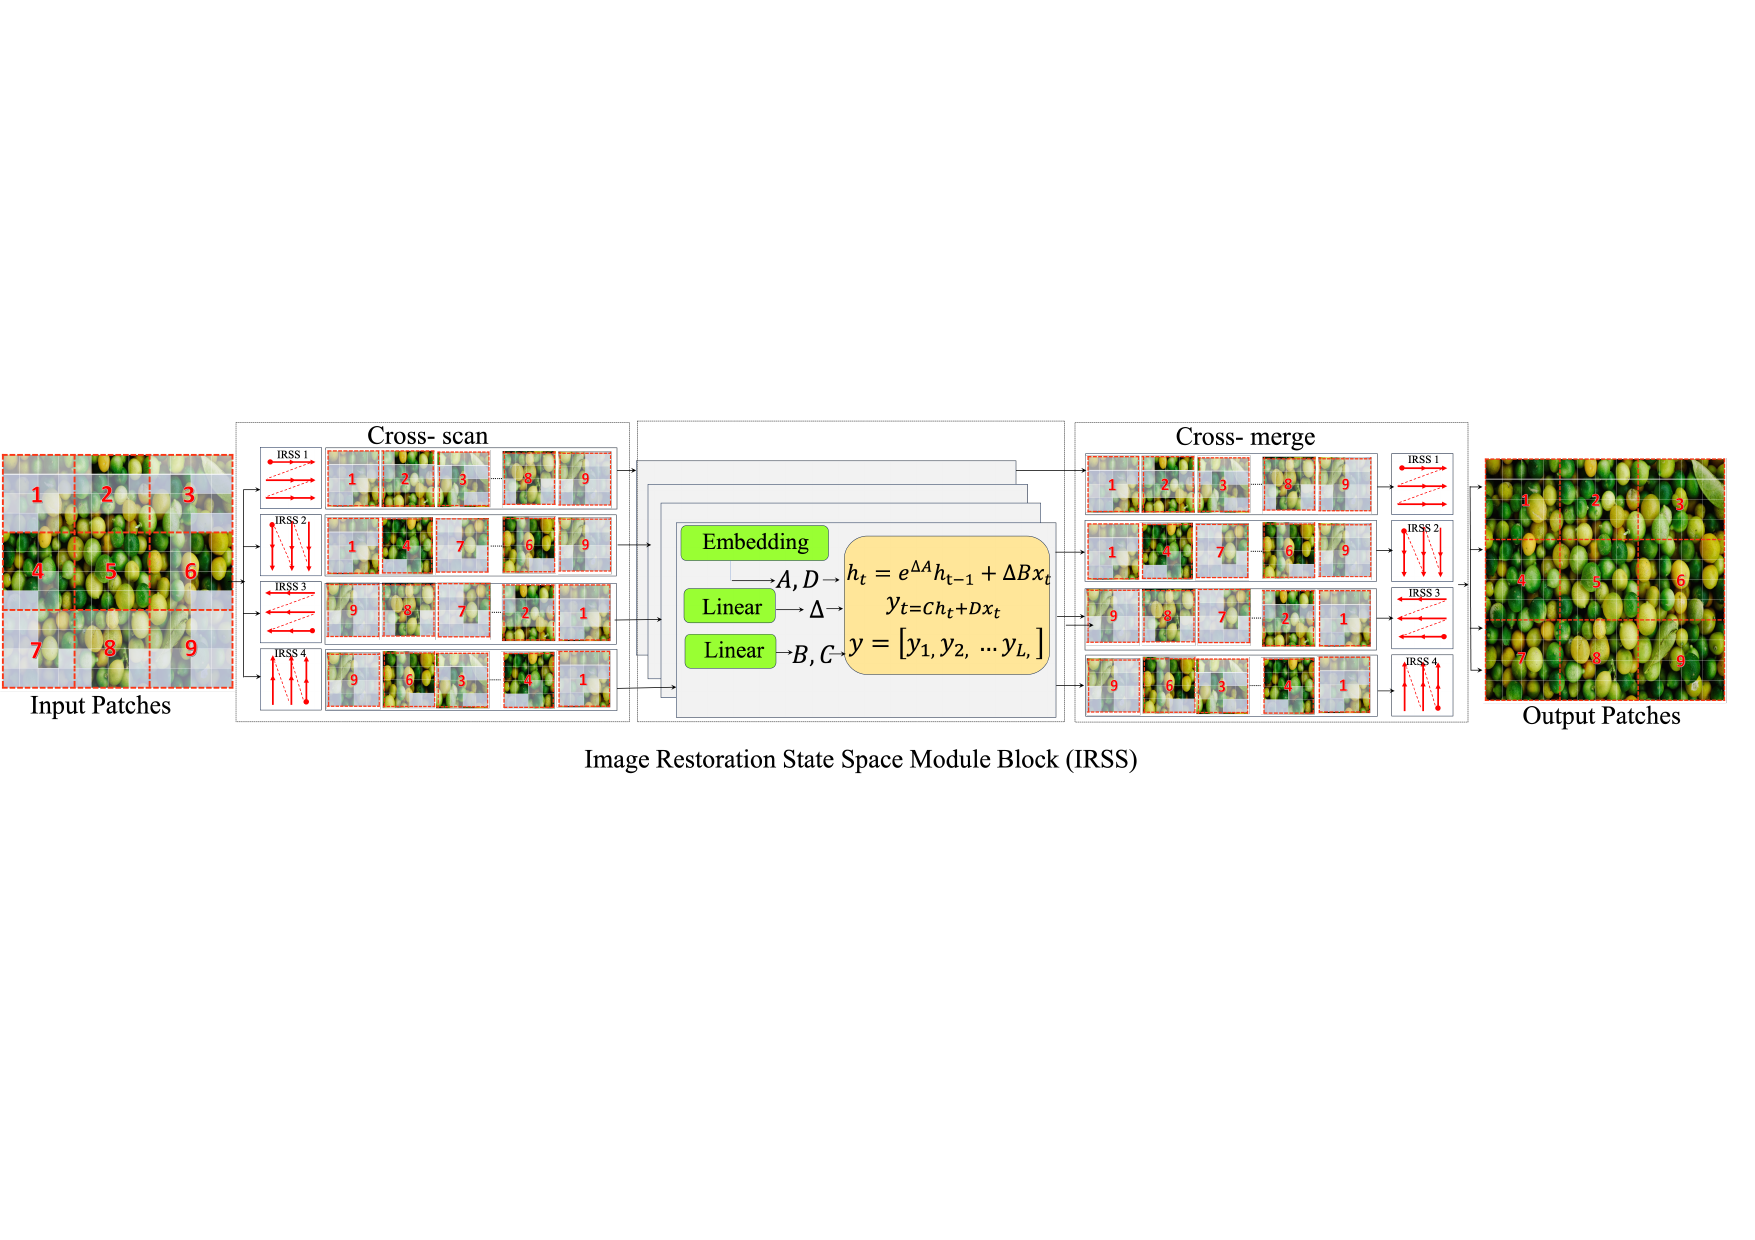}
    \vspace{-3mm}
    \caption{More details on IRSS, the core component of our MatIR model.}
    \label{fig:More details on IRSS}
    \vspace{4mm}
\end{figure*}

% \label{fig:comp_ir}
% \ref{fig:More details on IRSS}

\vspace{-6cm} 

\begin{table*}[t]
\arrayrulecolor[HTML]{DB5800}
\centering
\caption{Quantitative comparison on \underline{\textbf{classic image super-resolution}} with state-of-the-art methods. }
\label{tab:classicSR}
\setlength{\tabcolsep}{2pt}
\scalebox{0.92}{
\begin{tabular}{@{}l|c|cc|cc|cc|cc|cc@{}}
\toprule
 & & \multicolumn{2}{c|}{\textbf{Set5}} &
  \multicolumn{2}{c|}{\textbf{Set14}} &
  \multicolumn{2}{c|}{\textbf{BSDS100}} &
  \multicolumn{2}{c|}{\textbf{Urban100}} &
  \multicolumn{2}{c}{\textbf{Manga109}} \\
\multirow{-2}{*}{Method} & \multirow{-2}{*}{scale} & PSNR  & SSIM   & PSNR  & SSIM   & PSNR  & SSIM   & PSNR  & SSIM   & PSNR  & SSIM   \\ \midrule
MambaIR~\cite{guo2025mambair} & $\times 2$ &   38.57 & 0.9627& 34.67& 0.9261& 32.58 & 0.9048 & 34.15&    {0.9446} &   40.28 &   0.9806\\
CAT-A~\cite{chen2022cross} & $\times 2$ &     38.51 &   0.9626&    34.78&   0.9265&   32.59 &   0.9047 &   34.26&    {0.9440} &   40.10 &   0.9805\\
HAT~\cite{chen2023hat} & $\times 2$ &     38.63 &   0.9630&    34.86&   0.9274&   32.62 &   0.9053 &   34.45&    {0.9466} &   40.26 &   0.9809\\
ATD~\cite{zhang2024transcending}   & $\times 2$ & 38.61 & 0.9629 & 34.95 & 0.9276 & 32.65 & 0.9056 & 34.70 & 0.9476 & 40.37 & 0.9810 \\
GRL~\cite{li2023efficient}   & $\times 2$ & 38.67 & 0.9647 & 35.08 & 0.9303 & 32.67 & 0.9087 & 35.06 & 0.9505 & 40.67 & 0.9818 \\
{\textbf{MatIR (Ours)}}   & $\times 2$ &\fs{38.70}&\fs{0.9648}&\fs{35.13}&\fs {0.9304}&\fs{32.73}&\fs{0.9048}&\fs{35.11}& \fs {0.9507}&\fs{40.33}&\fs{0.9806} \\     \midrule
MambaIR~\cite{guo2025mambair} & $\times$3 &
   35.08&    0.9323 &    30.99 &    {0.8536} &    29.51 &    0.8157 &   {29.93} &    0.8841 &    35.43 &    0.9546\\
CAT-A~\cite{chen2022cross} & $\times$3 &
   35.06&    0.9326 &    31.04 &    {0.8538} &    29.52 &    0.8160 &   {30.12} &    0.8862 &    35.38 &    0.9546\\
HAT~\cite{chen2023hat} & $\times$3 &
   35.07&    0.9329 &    31.08 &    {0.8555} &    29.54 &    0.8167 &   {30.23} &    0.8896 &    35.53 &    0.9552\\
ATD~\cite{zhang2024transcending} & $\times$3 &
35.11 & 0.9330 & 31.13 & 0.8556 & 29.57 & 0.8176 & 30.46 & 0.8917 & 35.63 & 0.9558\\
{\textbf{MatIR (Ours)}}  & $\times$3 &  \fs{35.13} & \fs{0.9328} & \fs{31.06} & \fs{0.8555} & \fs{29.56} & \fs{0.8163} & \fs {30.23} & \fs{0.8888} & \fs{35.47} & \fs{0.9551}
\\ \midrule

MambaIR~\cite{guo2025mambair} & $\times 4$ &    33.03 &     0.9046 &     29.20 &    0.7961 &   27.98 &    0.7503 &    27.68 &   {0.8287} &     32.32 &     0.9272 \\
CAT-A~\cite{chen2022cross} & $\times 4$ &    33.08 &     0.9052 &     29.18 &    0.7960 &   27.99 &    0.7510 &    27.89 &   {0.8339} &     32.39 &     0.9285 \\
HAT~\cite{chen2023hat} & $\times 4$ &    33.04 &     0.9056 &     29.23 &    0.7973 &   28.00 &    0.7517 &    27.97 &   {0.8368} &     32.48 &     0.9292 \\
ATD~\cite{zhang2024transcending}   & $\times 4$ & 33.10 & 0.9058 & 29.24 & 0.7974 & 28.01 & 0.7526 & 28.17 & 0.8404 & 32.62 & 0.9306 \\
GRL~\cite{li2023efficient}   & $\times 4$ & 33.10 & 0.9094 & 29.37 & 0.8058 & 28.01 & 0.7611 & 28.53 & 0.8504 & 32.77 & 0.9325 \\
{\textbf{MatIR (Ours)}}   & $\times 4$ &\fs{33.14}&\fs{0.9055}&\fs{29.40}&\fs{0.8059}&\fs{28.03}&\fs{0.7610}&\fs{28.55}&\fs {0.8505}&\fs{32.82}&\fs{0.9326} \\  \bottomrule
\end{tabular}%
\label{table:table1}
}
\end{table*}

\begin{table}[h]
	\begin{center}
		\tabcolsep=0.13cm
		\singlespacing
		\vspace*{-4mm}
		\centering
		\captionsetup{justification=centering}
		\caption{Analysis of MatIR based on channel counts.}
		\vspace*{-3mm}
		\scalebox{1.0}{
			\begin{tabular}{cccc}
				\toprule
				\toprule
				Channels & Params (M) & Multi-Adds (G) & PSNR/SSIM \rule{0pt}{4ex} \\
				192 & 23.67 & 91.23 & 28.27dB/0.7584 \\
				\midrule
				180  & 19.01 & 69.39& 28.26dB/0.7583 \\
				\midrule
				144  & 13.35 & 39.43 & 28.13dB/0.7564 \\
				\midrule
				96  & 1.63  & 15.12 & 27.86dB/0.7489 \\
				\bottomrule
				\bottomrule
		\end{tabular}}
		\label{table:table2}
	\end{center}
	\vspace*{24.29mm}
\end{table}

\begin{table}[h]
	\begin{center}
		\tabcolsep=0.13cm
		\singlespacing
		\vspace*{-4mm}
		\centering
		\captionsetup{justification=centering}
		\caption{Analysis of MatIR based on model size.}
		\vspace*{-3mm}
		\scalebox{1.0}{
			\begin{tabular}{cccc}
				\toprule
				\toprule
				Models & Params (M) & Multi-Adds (G) & PSNR/SSIM \rule{0pt}{4ex} \\
				\midrule
				MatIR-l  & 34.89 & 97.08 & 28.56dB/0.7546 \\
				\midrule
				MatIR  & 22.07  & 69.39 & 28.26dB/0.7533 \\
				\midrule
				MatIR-s  & 14.35 & 39.43 & 28.06dB/0.7503 \\
				\midrule
				MatIR-r  & 3.98 & 38.64 & 27.99dB/0.7499 \\
				\bottomrule
				\bottomrule
		\end{tabular}}
		\label{table:table3}
	\end{center}
	\vspace*{30mm}
\end{table}

\vspace*{6mm}

\begin{figure*}[h]
	\centering
	\captionsetup{justification=centering}
	%\fbox{\rule{0pt}{2in} \rule{0.9\linewidth}{0pt}}
	\includegraphics[width=0.99\linewidth]{arXiv-2311.11600v1/figure/Polyline.pdf}
	\vspace*{-1mm}
	\caption{Comparison of iterative performance (PSNR in dB) of the proposed MatIR \textbf{Top-Left:} Performance comparison of triangle local attention, channel global attention and image recovery space modules. \textbf{Top-Right:} Triangle local attention and channel global attention, various interval sizes, \textbf{Bottom left:}
Different channel lengths. [On BSD100($\times4$), epoch 70]and \textbf{bottom right:}Performance evaluation of small, medium and large MatIR models.}
	% \vspace*{6mm}
	\label{fig:image_2}
\end{figure*}

\begin{figure*}[h]
	\centering
	\captionsetup{justification=centering}
	%\fbox{\rule{0pt}{2in} \rule{0.99\linewidth}{0pt}}
 \includegraphics[width=0.99\textwidth,height=0.5\textheight]{arXiv-2311.11600v1/figure/Barchart.pdf}
	\vspace*{-3mm}
	\caption{Comparison of various state-of-the-art models with MatIR on \textbf{Top-Left:} BSD100 (x2), \textbf{Top-Middle:} Urban100 (x3), \textbf{Top -Right:} Manga109 (x4), \textbf {Lower left:} Set14 (x4), \textbf{Lower middle:} Urban100 (x4), and \textbf{Bottom right:} Urban100 (x3).}
	\label{fig:image_3}
\end{figure*}

% Sec.\ref{fig:More details on IRSS}
% \label{fig:More details on IRSS}

% Tab. \ref{table:table2}
% \label{table:table2}

In this supplementary material, we provide more implementation details and visual results.First, we provide more implementation details in Section \cref{sec:More implementation details}.  
\\ Including
1. More details of IRSS, the core component of our MatIR model Fig. \ref{fig:More details on IRSS}. 
\\2. Classical SR quantitative comparison of our model and more SOTA models for image restoration Tab. \ref{table:table1}. 
\\3. Channel selection of our MatIR network architecture Tab. \ref{table:table2}.
\\4. Performance comparison of different scales of our MatIR network architecture Tab. \ref{table:table3}.
\\5. Model hyperparameter performance study Fig. \ref{fig:image_2}. 
\\6. We compare the performance of the proposed architecture with other state-of-the-art Transformer-based models and with a Mamba-based SR model Fig. \ref{fig:image_3}. 

Then, we provide more visual results of MatIR's Denoising, Defocus Deblurring qualitative comparison in Section \cref{sec:More visual results}.

\section{More implementation details}
\label{sec:More implementation details}

In this section, we study the impact of different hyperparameters and model core components on the performance of MatIR. We evaluate all model variants on the BSD100 dataset at different training iterations with a scaling factor of x4. We plot these results on the X-axis and their respective iterations on the Y-axis as shown in Fig. \ref{fig:image_2}. 
\\When we evaluate the model within the first 17.5k iterations, we find that there is a large deviation in the performance. Therefore, we adopt an averaging technique to keep the results stable at 5k, 7.5k, 10k, 12.5k, 15k, and 17.5k iterations. This averaging technique is implemented in the range of ±2.5k iterations or ±5 epochs. The leftmost chart shows the results of the model with channel global attention, triangle local attention and channel global attention, image inpainting state space (IRSS) module, triangle local attention and channel global attention. We find that the last configuration, namely our proposed MatIR, produces the best results. It also shows the importance of our core module relative to the regular attention model. The right chart justifies the choice of interval size "2" instead of other interval sizes. The bottom left figure plots the model results for three channel counts (180, 144, and 96). Performance of three CFAT variants: CFAT-1, CFAT, and CFAT-s. Based on the performance in the bottom-middle figure, we determine the best combination of window sizes for rectangular and triangular window attention. We plot the performance of three CFAT variants in the bottom-right figure: model results of CFAT-1, CFAT, and CFAT-s.

\section{More visual results}
\label{sec:More visual results}

See Fig. \ref{fig:image_4}, Fig. \ref{fig:image_5} for details.

\begin{figure*}
    \centering
    
    \captionsetup{font={small}} 
    
    \includegraphics[width=.99\linewidth]{arXiv-2311.11600v1/figure/Denoising.pdf}

    \vspace{-3mm}
    \caption{Visual comparisons between MatIR and state-of-the-art Denoising methods.}
    \label{fig:image_4}
    \vspace{-3mm}
\end{figure*}

\begin{figure*}
    \centering
    
    \captionsetup{font={small}} 
    
    \includegraphics[width=.99\linewidth]{arXiv-2311.11600v1/figure/Defocus_Deblurring.pdf}

    \vspace{-3mm}
    \caption{Visual comparisons between MatIR and state-of-the-art Defocus Deblurring methods. }
    \label{fig:image_5}
    \vspace{-3mm}
\end{figure*}

\begin{figure*}[t]
  \centering
   \vspace{-0.5mm}
   \includegraphics[width=1\linewidth]{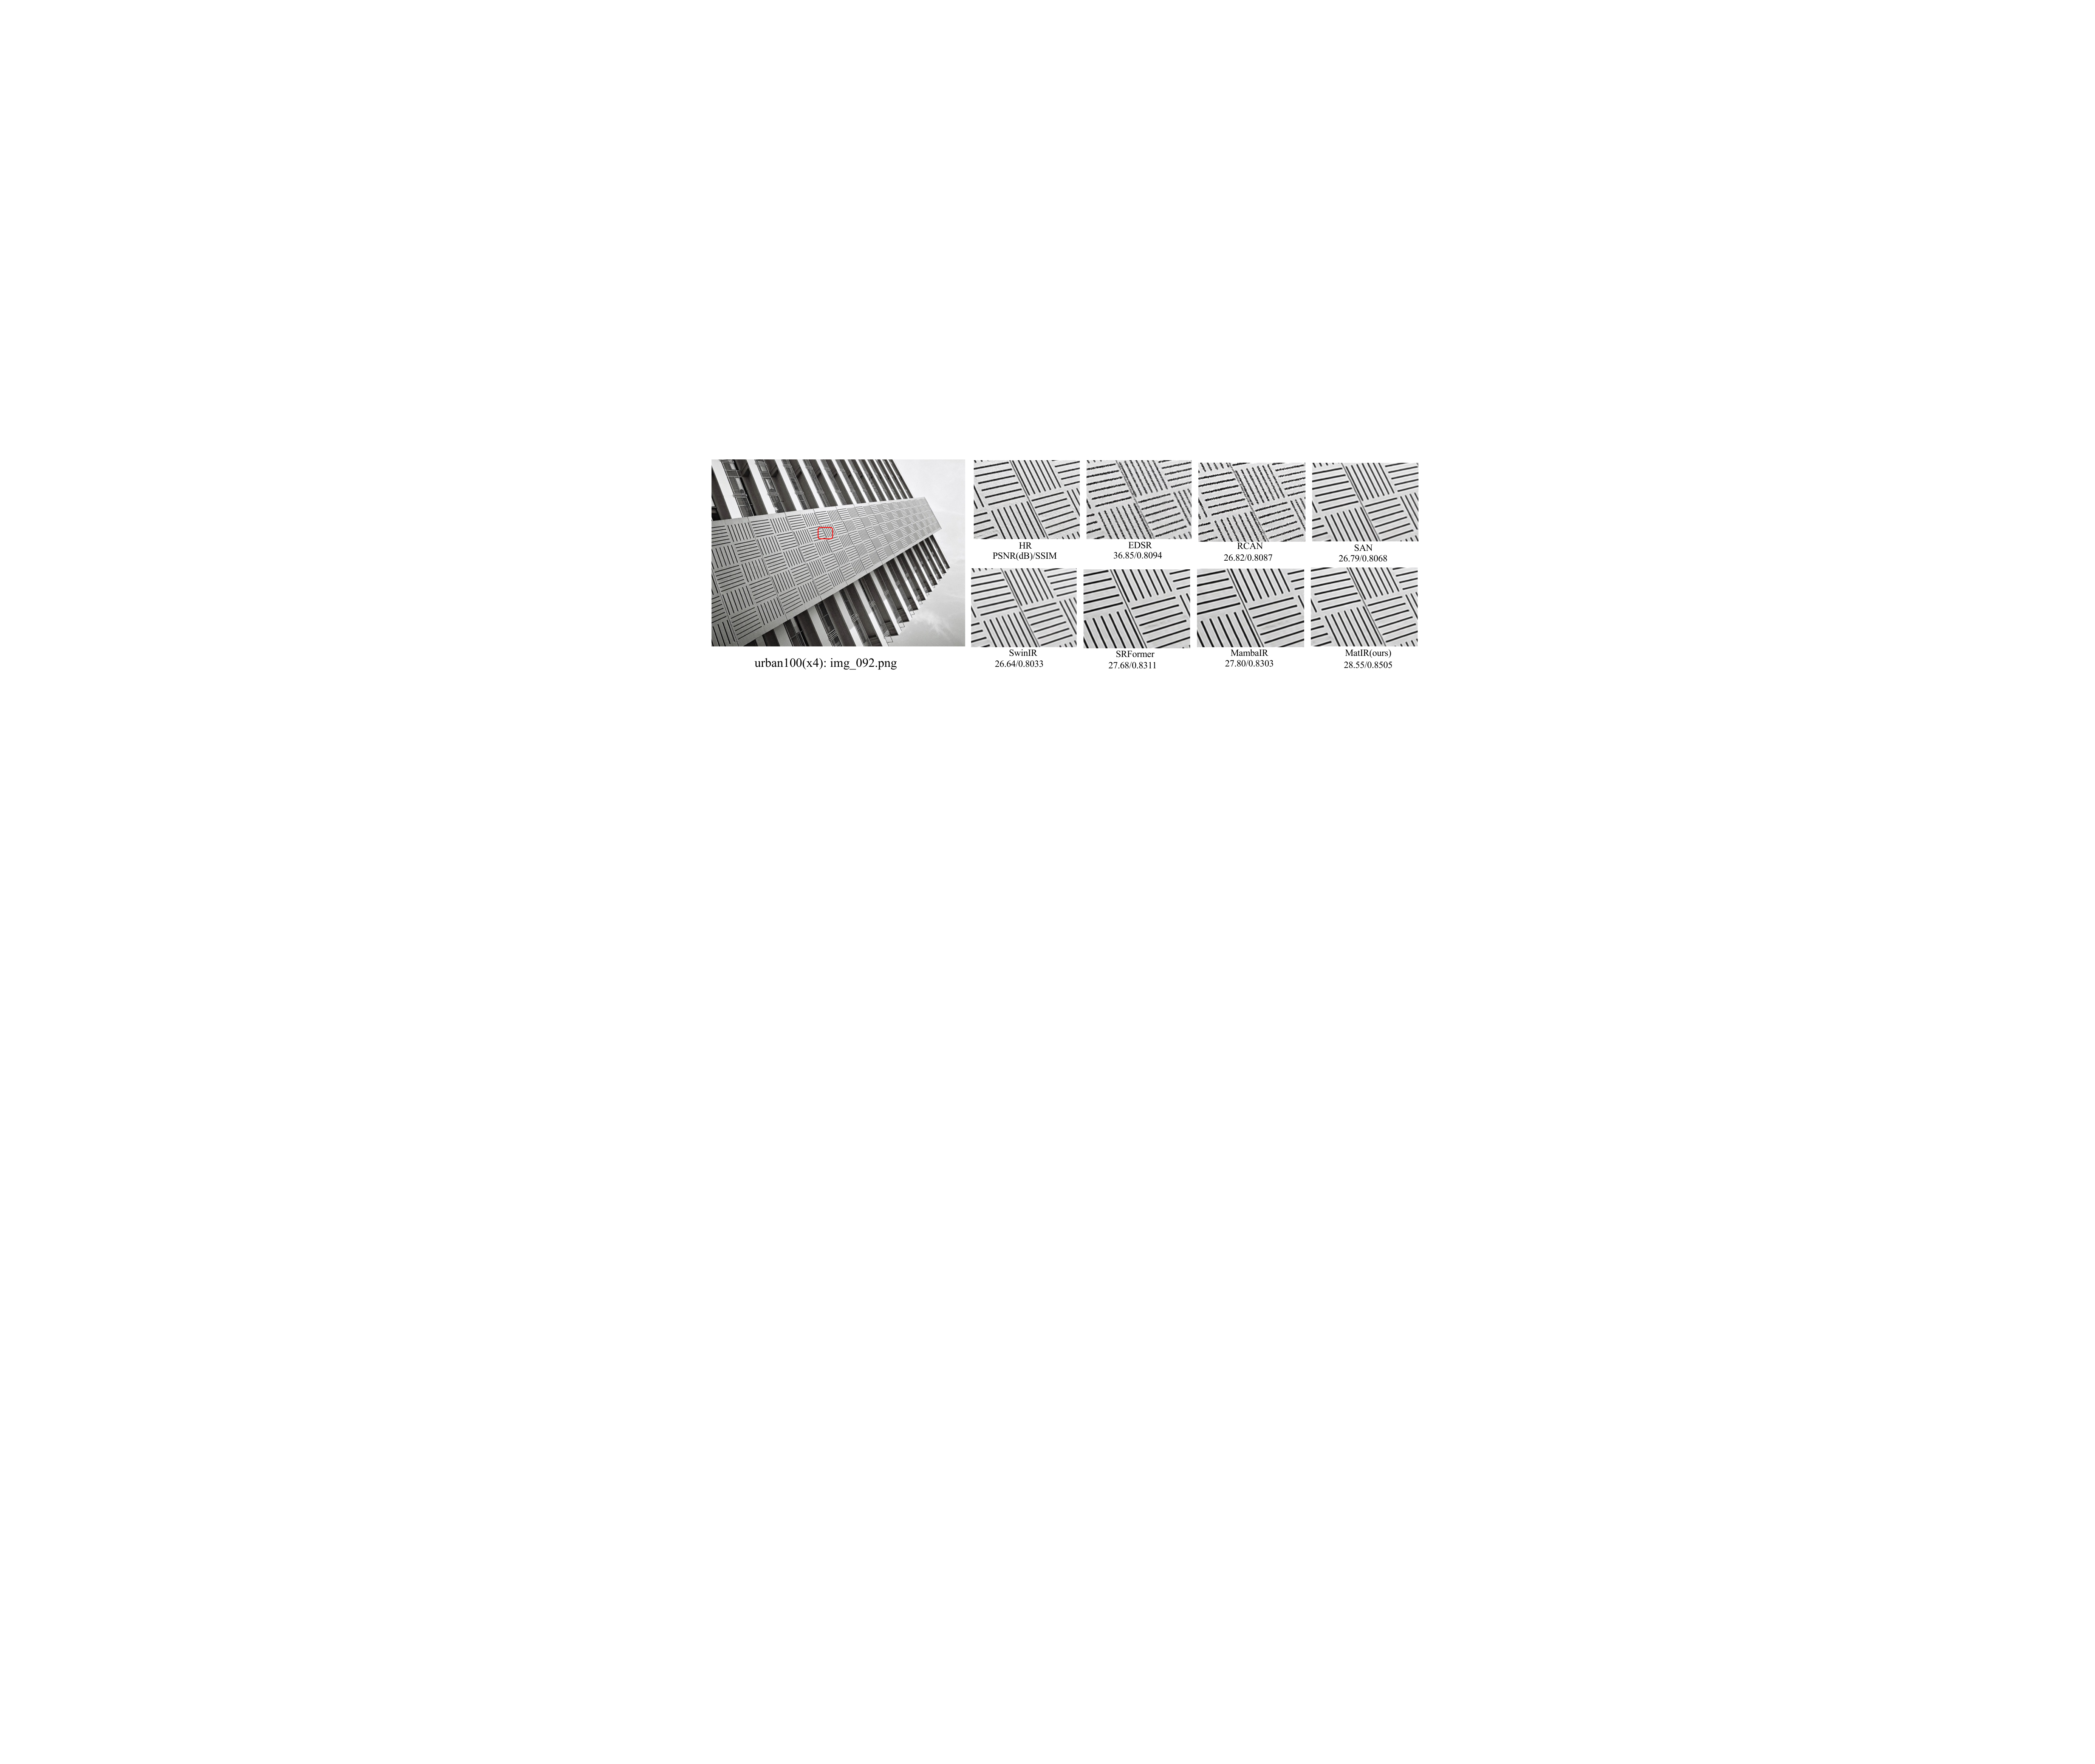}
   \vspace{-7mm}
   \caption{The visual comparison of the MatIR network on x4SR utilizes red bounding boxes to highlight the patch for comparison, in order to better reflect performance differences.}
   \vspace{-6mm}
   \label{fig:x4sr}
\end{figure*}
